# Supplementary material for: BloomGML: Graph Machine Learning through the Lens of Bilevel Optimization
Source: arXiv:2403.04763 source file (2024-03-07)
Supplement: Supplementary file 2 [file general_fU.tex]

\section{Attempt of a tighter $\hat{f}_U$}

Given a message-passing GNN layer expressed as 

\begin{equation}
    \h{l} = \h{l-1} - 
\end{equation}
