# Supplementary material for: BloomGML: Graph Machine Learning through the Lens of Bilevel Optimization
Source: arXiv:2403.04763 source file (2024-03-07)
Supplement: Supplementary file 3 [file nbfnet_proof.tex]

\section{}
